# Supplementary material for: Self-similar orbit-averaged Fokker-Planck equation for isotropic spherical dense clusters (i) accurate pre-collapse solution
Source: arXiv:2003.12196 source file (2020-04-30)
Supplement: Supplementary file 1 [file Appendix_Radau.tex]

\section{Radau nodes}

the Gauss-Radau nodes 
\begin{subequations}
\begin{align}
t_{k}=\frac{2k-2}{2N-1}
\end{align}
\end{subequations}
and

the orthogonality conditions (e.g. \cite{Mason_2002})  for Radau nodes
\begin{equation}
\sum^{N}_{j=1}{}^{\prime\prime} T_{n}(x_j)T_{m}(x_j)=\left\{\begin{matrix}
&0&\\
&\frac{2N-1}{2}&\\
&\frac{2N-1}{4}&
\end{matrix}\right.\hspace{1cm}
\begin{matrix}
&(1<n\neq m<N)&\\
&(n=m=0)&\\
&(0<n=j\leq N)&
\end{matrix}
\end{equation}
where the double prime indicates that the 1st term of the summation must be divided by $2$.

The Chebyshev-Radau expansion can be inverted to
\begin{subequations}
	\begin{align}
	&a_{1}=\frac{2}{2N-1}\sum^{N}_{j=1}{}^{\prime\prime}T_{0}(x_{j})f(x_j)\label{DCC1}\\
	&a_{n}=\frac{4}{2N-1}\sum^{N}_{j=1}{}^{\prime\prime}T_{n-1}(x_{j})f(x_j). \label{DCC2} \hspace{1cm}2\leq n\leq N
	\end{align}
\end{subequations}
